# Supplementary material for: Identifying inflated super-Earths and photo-evaporated cores
Source: arXiv:1804.05069 source file (2018-09-05)
Supplement: Supplementary file 1 [file appendix-table.tex]

\section{Inflated super-Earths}
\label{appendix:inflated}

\begin{table}[h!]\label{tab:inflated}
  \caption{These are the super-Earth pairs with the most extreme radius ratios. All the pairs have radius ratio $R_{\rm out} / R_{\rm in} > 2.3$ and straddle both of the candidate $R_{\rm trans}$ lines shown in Figure \ref{fig:radius-Flux-v2}. In section \ref{sec:results:inflated} we argue that in these systems the outer planet probably has an inflated atmosphere. The first column shows the KOI number of each planet. $T_{\rm eff}$ and $R_\star$ are the effective temperature and the radius of the star.}
  \begin{tabular}{lrcrccr|rlrcrcc}
  KOI & $P\;\;\;\;$ & $R$ & $\Teq\;\;$ & $T_{\rm eff}$ & $R_\star$ & $$ & $$ & KOI & $P\;\;\;\;$ & $R$ & $\Teq\;\;$ & $T_{\rm eff}$ & $R_\star$ \\
  \hline
  K00112.02  &    3.709d  &  1.16$\Re$  &  1206K  &  5833K  &  1.02$R_\odot$ &
  $\;$ & $\;$ &
  K00117.04  &    7.958d  &  1.06$\Re$  &  1074K  &  5847K  &  1.40$R_\odot$ \\
  K00112.01  &   51.079d  &  2.75$\Re$  &   503K  &  5833K  &  1.02$R_\odot$ &
  $\;$ & $\;$ &
  K00117.01  &   14.749d  &  2.89$\Re$  &   874K  &  5847K  &  1.40$R_\odot$ \\
  \hline
  K01557.04  &    1.499d  &  1.09$\Re$  &  1137K  &  4723K  &  0.69$R_\odot$ &
  $\;$ & $\;$ &
  K01628.02  &    1.772d  &  1.02$\Re$  &  1685K  &  6243K  &  1.15$R_\odot$ \\
  K01557.01  &    3.296d  &  2.81$\Re$  &   875K  &  4723K  &  0.69$R_\odot$ &
  $\;$ & $\;$ &
  K01628.01  &   19.747d  &  2.62$\Re$  &   754K  &  6243K  &  1.15$R_\odot$ \\
  \hline
  K01522.02  &   12.655d  &  1.02$\Re$  &   801K  &  5833K  &  1.02$R_\odot$ &
  $\;$ & $\;$ &
  K01598.03  &   13.931d  &  1.40$\Re$  &   665K  &  5497K  &  0.84$R_\odot$ \\
  K01522.01  &   33.386d  &  2.48$\Re$  &   580K  &  5833K  &  1.02$R_\odot$ &
  $\;$ & $\;$ &
  K01598.01  &   56.476d  &  3.22$\Re$  &   417K  &  5497K  &  0.84$R_\odot$ \\
  \hline
  K01480.02  &    7.004d  &  1.19$\Re$  &   754K  &  4883K  &  0.81$R_\odot$ &
  $\;$ & $\;$ &
  K02034.02  &    2.370d  &  1.29$\Re$  &  1256K  &  5668K  &  0.87$R_\odot$ \\
  K01480.01  &   20.382d  &  3.16$\Re$  &   528K  &  4883K  &  0.81$R_\odot$ &
  $\;$ & $\;$ &
  K02034.01  &    3.609d  &  3.26$\Re$  &  1092K  &  5668K  &  0.87$R_\odot$ \\
  \hline
  K01831.03  &   34.206d  &  1.10$\Re$  &   471K  &  5191K  &  0.83$R_\odot$ &
  $\;$ & $\;$ &
  K01899.02  &   10.523d  &  1.08$\Re$  &   976K  &  6327K  &  1.18$R_\odot$ \\
  K01831.01  &   51.810d  &  2.60$\Re$  &   410K  &  5191K  &  0.83$R_\odot$ &
  $\;$ & $\;$ &
  K01899.01  &   19.762d  &  2.81$\Re$  &   791K  &  6327K  &  1.18$R_\odot$ \\
  \hline
  K01986.02  &    7.128d  &  1.21$\Re$  &   784K  &  5159K  &  0.82$R_\odot$ &
  $\;$ & $\;$ &
  K02449.02  &    0.912d  &  1.46$\Re$  &  1840K  &  5481K  &  1.04$R_\odot$ \\
  K01986.01  &  148.460d  &  3.61$\Re$  &   285K  &  5159K  &  0.82$R_\odot$ &
  $\;$ & $\;$ &
  K02449.01  &   53.358d  &  3.41$\Re$  &   474K  &  5481K  &  1.04$R_\odot$ \\
  \hline
  K00282.02  &    8.457d  &  1.02$\Re$  &   982K  &  5903K  &  1.14$R_\odot$ &
  $\;$ & $\;$ &
  K03130.02  &    5.652d  &  1.05$\Re$  &   856K  &  5159K  &  0.80$R_\odot$ \\
  K00282.01  &   27.509d  &  2.98$\Re$  &   663K  &  5903K  &  1.14$R_\odot$ &
  $\;$ & $\;$ &
  K03130.01  &   14.864d  &  2.90$\Re$  &   620K  &  5159K  &  0.80$R_\odot$ \\
  \hline
  K00584.03  &    6.470d  &  1.15$\Re$  &   926K  &  5475K  &  0.98$R_\odot$ &
  $\;$ & $\;$ &
  K00547.03  &   12.386d  &  1.11$\Re$  &   679K  &  5121K  &  0.89$R_\odot$ \\
  K00584.01  &    9.927d  &  2.76$\Re$  &   803K  &  5475K  &  0.98$R_\odot$ &
  $\;$ & $\;$ &
  K00547.01  &   25.303d  &  3.95$\Re$  &   535K  &  5121K  &  0.89$R_\odot$ \\
  \hline
  K00094.04  &    3.743d  &  1.50$\Re$  &  1423K  &  6181K  &  1.33$R_\odot$ &
  $\;$ & $\;$ &
  K00459.02  &    6.920d  &  1.39$\Re$  &   961K  &  5815K  &  0.95$R_\odot$ \\
  K00094.02  &   10.424d  &  3.72$\Re$  &  1012K  &  6181K  &  1.33$R_\odot$ &
  $\;$ & $\;$ &
  K00459.01  &   19.446d  &  3.24$\Re$  &   681K  &  5815K  &  0.95$R_\odot$ \\
  \hline
  K00408.04  &    3.428d  &  1.21$\Re$  &  1131K  &  5559K  &  0.91$R_\odot$ &
  $\;$ & $\;$ &
  K00471.02  &    7.811d  &  1.36$\Re$  &   906K  &  5395K  &  1.07$R_\odot$ \\
  K00408.01  &    7.382d  &  3.42$\Re$  &   876K  &  5559K  &  0.91$R_\odot$ &
  $\;$ & $\;$ &
  K00471.01  &   21.347d  &  3.20$\Re$  &   648K  &  5395K  &  1.07$R_\odot$ \\
  \hline
  K00691.02  &   16.225d  &  1.21$\Re$  &   788K  &  5956K  &  1.10$R_\odot$ &
  $\;$ & $\;$ &
  K03500.02  &    4.748d  &  1.57$\Re$  &  1690K  &  6056K  &  2.48$R_\odot$ \\
  K00691.01  &   29.666d  &  2.83$\Re$  &   644K  &  5956K  &  1.10$R_\odot$ &
  $\;$ & $\;$ &
  K03500.01  &   73.750d  &  3.78$\Re$  &   677K  &  6056K  &  2.48$R_\odot$
  \end{tabular}
\end{table}
